# Supplementary material for: Comparing verbal, visual and combined explanations for Bayesian Network inferences
Source: arXiv:2511.16961 source file (2026-11-27)
Supplement: Supplementary file 1 [file Appendix-QTdefinitions.tex]

\subsection{Terminology}

\begin{itemize}
    
\item \textbf{“the target state”} Our tool explains the difference evidence makes to the probability of a particular variable state we are interested in. Of course, this state is different in different test BNs, so our generic term is “target” state. Our question category definitions for experimenter use must use this term to be independent of any particular test BN. 
\item \textbf{“a finding’s contribution”} We define these 3 words to mean these 15 words: “the difference learning the finding makes to the target probability, given all the other findings”. (As with “target”, we usually avoid this technical term in the experiment.).
\item \textbf{“hypothetical scenario”} is “a situation that is not displayed in which the set of findings is different”.
\end{itemize}

Criteria for categorizing Expt 1 questions
Which knowledge or skill does the participant need in order to reliably answer the question correctly?

\subsection{Definitions}

\textbf{Finding:} Know something about the contributions of the findings in the actual scenario (e.g. whether they increase or decrease the target’s probability, or which finding’s contribution is bigger).

\textbf{Path:} Know the difference this path makes to the finding’s contribution.

\textbf{Path what-if:} Be able to imagine a new hypothetical scenario, and be able to work out which paths would now be active. Using information provided by our markup for the paths in the actual scenario, be able to infer something about the finding’s new contribution.

\textbf{Control Path what-if:} Be able to imagine a new hypothetical scenario, and be able to work out which paths would now be active. Be able to infer something about the finding’s new contribution. (Information provided by our actual path markup is not necessary.)

\textbf{Control:} Knowing any information provided only by our markup is not necessary.

\textbf{Common effect what-if:} Know one of these aspects of the common effect relationship, which are all finding contributions in hypothetical scenarios. (In our experiment, one of the causes is the target, and in the actual scenario we have findings about the effect and the other cause.)
(a) if we didn't know about the effect or either cause, know something about how finding out about each cause (or both) would change the probability of the effect
(b) if we didn't know about the effect or either cause, know something about how the finding about one cause would change the probability of the target (the other cause)
(c) if we didn't know about the other cause or the effect, know something about how finding out about the effect would change the probability of the target
