# Supplementary material for: Comparing verbal, visual and combined explanations for Bayesian Network inferences
Source: arXiv:2511.16961 source file (2026-11-27)
Supplement: Supplementary file 2 [file Appendix-Participants.tex]

\input tables/tab-results-distribution
